# Supplementary material for: PuzzlePlex: Benchmarking Foundation Models on Reasoning and Planning with Puzzles
Source: arXiv:2510.06475 source file (2025-10-07)
Supplement: Supplementary file 1 [file appendix.tex]

\section{Appendix}
