# Supplementary material for: PuzzlePlex: Benchmarking Foundation Models on Reasoning and Planning with Puzzles
Source: arXiv:2510.06475 source file (2025-10-07)
Supplement: Supplementary file 2 [file appendix_tmp_per_puzzle_singleplayer.tex]

\begin{table}[t]
\caption{Performance comparison of large language models on three single-player deterministic puzzles. Scores are reported in Elo ratings for both Easy and Normal difficulty settings. The top three performing models for each task and difficulty are highlighted (\colorbox{red!35}{first}, \colorbox{red!20}{second}, and \colorbox{red!5}{third} place). }
\label{tab:selected_puzzles}
\centering
\begin{tabular}{lcccccc}
\toprule
\multirow{2}{*}{\textbf{Model}} &
\multicolumn{2}{c}{\textbf{TidyTower}} &
\multicolumn{2}{c}{\textbf{OptimalTouring}} &
\multicolumn{2}{c}{\textbf{CountMaximalCocktails}} \\
\cmidrule(lr){2-3}  \cmidrule(lr){4-5} \cmidrule(lr){6-7}
 & Easy & Normal & Easy & Normal & Easy & Normal\\
\midrule
\textbf{Custom} & {1481.3} & {1464.0} & {1098.1} & {1047.6} & {1173.2} & {1178.2} \\
\midrule
\textbf{o4-mini} & 956.1 & 952.8 & \cellcolor{red!35}{1350.1} & \cellcolor{red!35}{1421.3} & 978.4 & {985.8} \\
\textbf{Deepseek-r1} & 956.2 & 952.4 & \cellcolor{red!20}{1312.6} & \cellcolor{red!20}{1251.6} & \cellcolor{red!35}{1170.9} & \cellcolor{red!35}{1048.8} \\
\textbf{Deepseek-V3} & 956.2 & 952.2 & {1004.8} & 914.1 & 979.7 & 985.8 \\
\textbf{GPT-4.1} & 956.1 & 953.0 & 1190.8 & \cellcolor{red!5}{1190.9} & 978.4 & 983.8 \\
\textbf{grok-3-mini} & 956.2 & 952.5 & 712.7 & 794.3 & 978.2 & 986.5 \\
\textbf{Gemini-2.5-pro} & 956.1 & 952.7 & \cellcolor{red!5}{1311.8} & 1146.5 & 978.3 & \cellcolor{red!20}{1039.8} \\
\textbf{QwQ-32B} & 956.3 & 952.0 & 1168.7 & 1110.3 & \cellcolor{red!20}{1097.2} & 902.4 \\
\textbf{Qwen-2.5-VL-72B} & \cellcolor{red!35}{956.4} & \cellcolor{red!35}{1012.7} & 746.0 & 819.8 & \cellcolor{red!5}{1013.2} & \cellcolor{red!5}{1019.8} \\
\textbf{Llama-3.3-70B} & 956.3 & 951.9 & 686.0 & 768.3 & 947.5 & 955.5 \\
\textbf{Gemma-3-27B} & \cellcolor{red!35}{956.4} & 951.8 & 674.1 & 819.0 & 946.1 & 984.2 \\
\textbf{Phi-4-multimodal} & 956.3 & 952.1 & 744.4 & 716.5 & 758.9 & 929.4 \\
\bottomrule
\end{tabular}
\end{table}
